# Supplementary material for: Interpretable, similarity-driven multi-view embeddings from high-dimensional biomedical data
Source: arXiv:2006.06545 ancillary file (2021-01-21)
Supplement: Supplementary file 1 [file supp_info_1.pdf]

# SiMLR Supplementary Information

Brian B. Avants, Nicholas J. Tustison, James R. Stone

## 1 Supplementary Figures

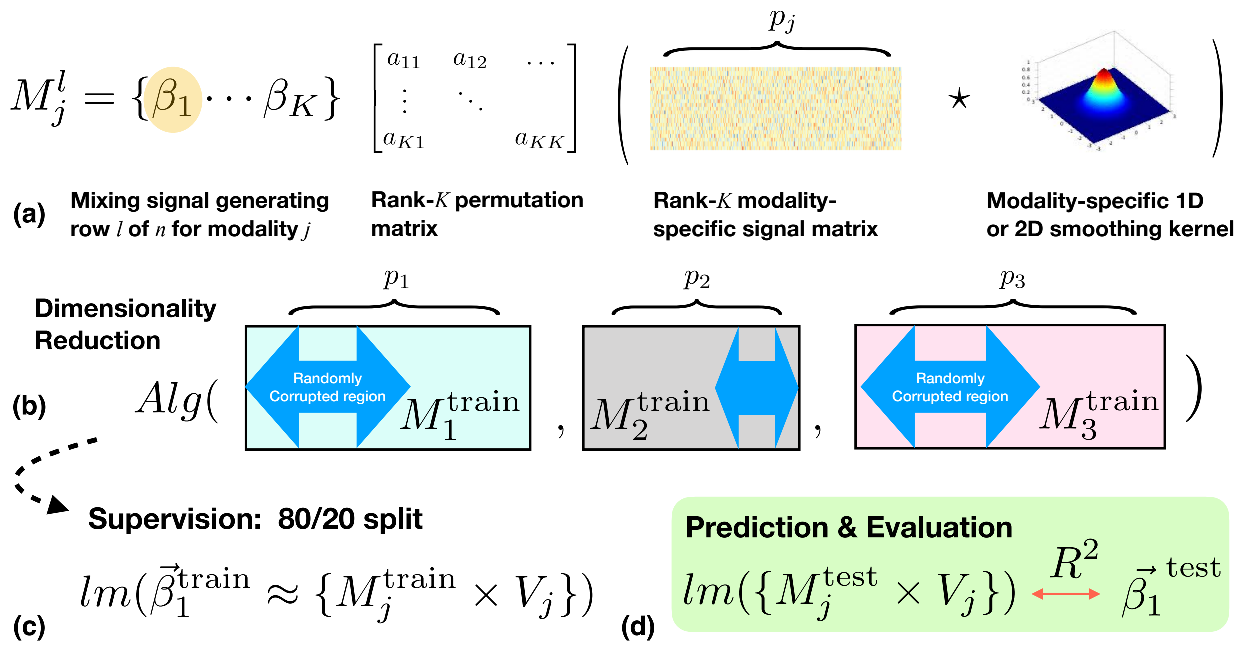


Supplementary Figure 1: Conceptual overview of the SiMLR simulation study which defines an inverse problem for signal recovery with known ground truth. (a) shows the generation of a given row, $M_j^l$, in a single simulated matrix, $M_j$. The $K$-rank generating basis set is smoothed to induce signal-specific covariation as is present in many types of real biological data. The highlighted beta is the common signal that we seek to recover. (b) The study also randomly corrupts each of the three generated matrices by eliminating any true signal in some fraction of the matrix. The fraction of corruption is drawn from a uniform distribution between 0.1 and 0.9 (i.e. 10 and 90 percent corruption). (c) We define a random 80/20 split for each simulation and learn from the 80 percent of training data. RGCCA, SGCCA and SiMLR are each run in the dimensionality reduction step. A linear regression method then fits the low-dimensional embeddings to the ground truth signal in the training data. (d) This process enables us to evaluate the signal recovery performance in the test set and how it is impacted by the corruption process.

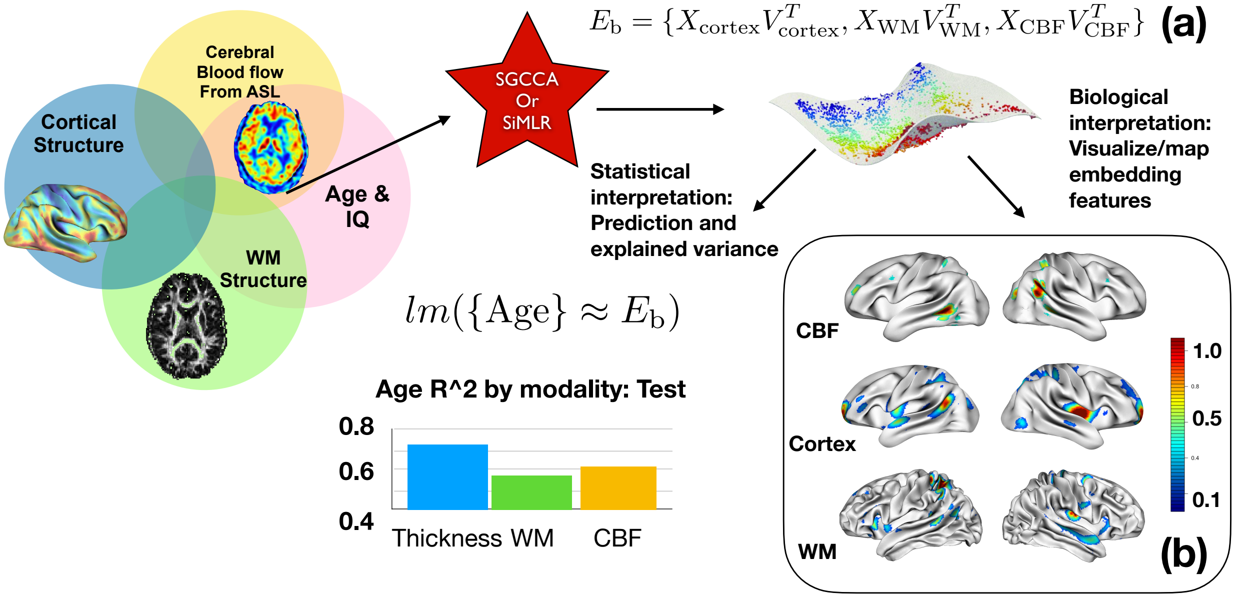


Supplementary Figure 2: PTBP fully supervised brain age prediction: comparison to SGCCA. Brain age is the subject's age predicted from neuroimaging data. Four matrices are input where cortical thickness, white matter integrity and cerebral blood flow derive from different types of neuroimages; the fourth modality describes brain maturation in terms of age and IQ measurements. Panel (a) shows the overall study design where embeddings are computed as in prior examples and then passed downstream to facilitate statistical and biological interpretation. The first phase of statistical interpretation ( the bar plots ) compares the ability of each modality to predict age independently and suggests thickness is most predictive (when acting alone); WM and CBF have close performance to each other (data drawn from best performing method). In (b), we show the feature vectors from the best performing method noting that the weights are relative to each feature vector where its values are scaled to zero to one.

# 2 Pediatric imaging genomics

The key to this application demonstration is a recently reported analysis of genetic risk variants in depression[1]. Wray, et. al. provide chromosomal regions for 44 genetic loci associated with depression based on a large collection of data (135,458 subjects with major depression and 344,901 controls). This report allowed us to extract SNPs from these regions in an independent pediatric dataset (PING, described below[2]) which also provides neuroimaging and, in a subset of subjects, clinical depression and anxiety scores. SiMLR will relate PING genotype to imaging phenotype and produce an embedding — from subjects without depression scores — that may be tested for predictive power in separate subjects that do have depression scores. The *testing* sample in no way overlaps with the training sample, although these subjects are selected from the same overall PING cohort.

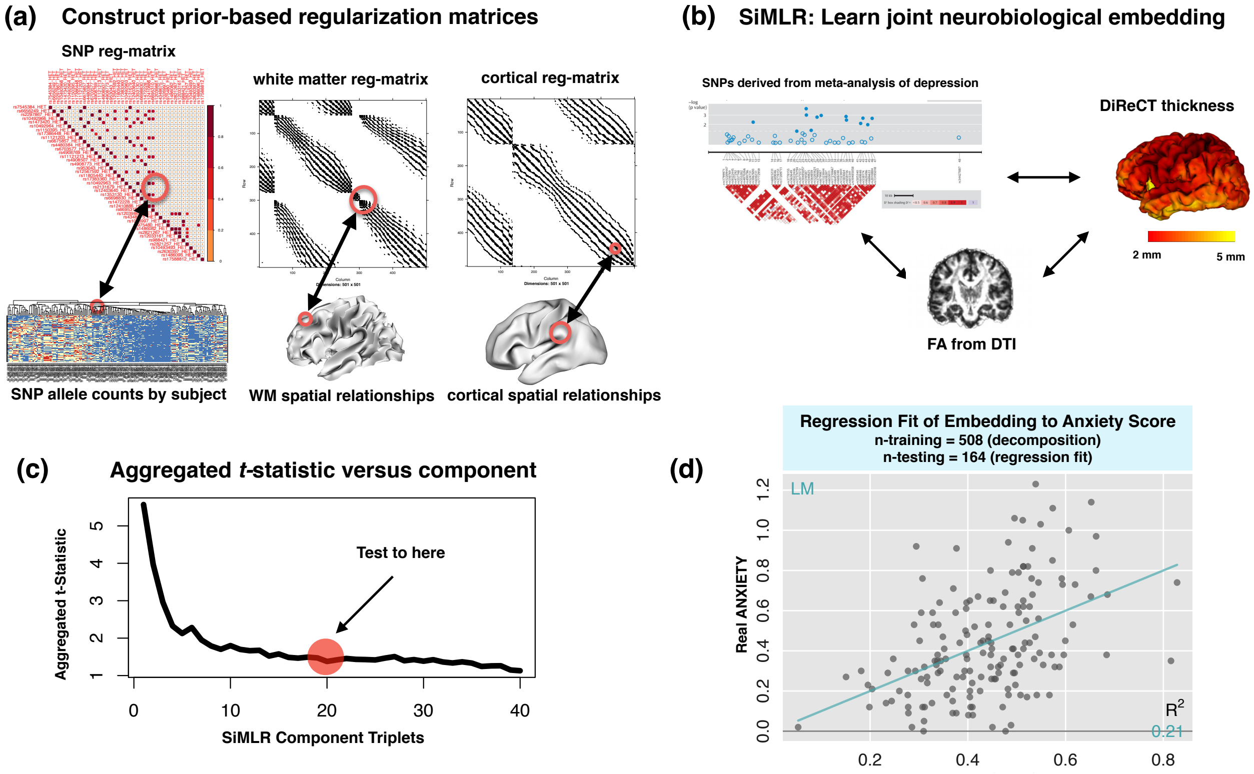


Supplementary Figure 3: Depression and imaging genomics study overview. Panel (a) identifies the nature of the regularization used here, i.e. spatial regularization based on the cortical and white matter manifolds and regularization based on linkage disequilibrium for the SNP data. Panel (b) provides a visual representation of the learning process. Panel (c) demonstrates our selection process for the number of embeddings to test against anxiety and depression scores. Panel (d) shows the multi-view prediction results for anxiety based on thickness, FA and SNP embedding vectors applied in testing data. The thickness and SNP based embeddings contribute the most. The fit to depression scores is similar though less significant under permutation tests.

## 2.1 Data availability

Data used in the preparation of this article were obtained from the Pediatric Imaging, Neurocognition and Genetics (PING) Study database (https://chd.ucsd.edu/research/ping.html and https://ndar.nih.gov/edit_collection.html?id=2607). PING was launched in 2009 by the National Institute on Drug Abuse (NIDA) and the Eunice Kennedy Shriver National Institute Of Child Health & Human Development (NICHD) as a 2-year project of the American Recovery and Reinvestment Act. The primary goal of PING has been to create a data resource of highly standardized and carefully curated magnetic resonance imaging (MRI) data, comprehensive genotyping data, and developmental and neuropsychological assessments for a large cohort of developing children aged 3 to 20 years. The scientific aim of the project is, by openly sharing these data, to amplify the power and productivity of investigations of healthy and disordered development in children, and to increase understanding of the origins of variation in neurobehavioral phenotypes. For up-to-date information, see https://chd.ucsd.edu/research/ping.html. Data collection and sharing for this project was funded by the Pediatric Imaging, Neurocognition and Genetics Study (PING) (National Institutes of Health Grant RC2DA029475). PING is funded by the National Institute on Drug Abuse and the Eunice Kennedy Shriver National Institute of Child Health & Human Development. PING data are disseminated by the PING Coordinating Center at the Center for Human Development, University of California, San Diego.

For this example analysis, we divided the $n = 670$ PING subjects into training and testing based on a simple criterion: the availability of self-report measurements. The training cohort ($n = 508$) did not have such scores but did have imaging, genetic and other measurements. The age-matched testing ($n = 164$) group had completed both a summary clinical measurement of anxiety (Screen for Child Anxiety Related Emotional Disorders – Revised (AED)) and a second measurement of depression (Center for Epidemiological Studies Depression Scale for Children (CES-DC)). Table 1 shows relevant demographic variables for this split cohort. All subjects in both training and testing had three additional measurements: dense voxel-wise measurements of cortical thickness (derived from ANTs tools, v2.2.0 and following[3,4]), dense voxel-wise measurements of fractional anisotropy in white matter as well as a set of SNPs associated with depression via prior genome-wide meta analysis[1]. The normalized cortical thickness and FA images contain 66,565 and 68,966 voxels, respectively. We extracted 4,309 candidate SNPs from imputed PING data using default settings of the open-source software Plink[5]. Many of these SNPs exhibit known associations with neural processes and/or brain development, as described in annotations provided by[1]. As such, we refer the reader to that document for interpretation of the involved SNPs in the appropriate broader context.

Supplementary Table 1: Demographics Table: The table details group characteristics for primary covariates in the training and testing groups. No significant differences exist. Note that depression and anxiety measures are only available within the testing group.

| Predictor | trainGroup | testGroup | pValue |
|---|---|---|---|
| Age | 14.6 ± 3.9 | 14.2 ± 3.8 | 0.338 |
| Gender=F/M | 240 (47.2%)/268 | 82 (50.0%)/82 | 0.6 |
| parental education | 5.7 ± 1.2 | 5.9 ± 1.1 | 0.06 |
| parental income | 6.8 ± 2.5 | 7.1 ± 2.3 | 0.11 |
| CES-DC | NA | 0.7 ± 0.5 | NA |
| AED | NA | 0.44 ± 0.27 | NA |

*Regularization matrices:* For the cortical and FA data, we employ a sparse gaussian regularization matrix, shown in Figure 3, that is based on spatial proximity along the cortical and white matter manifolds, respectively, as in previous studies[6]. This matrix is constructed automatically, given the sigma of the desired gaussian. For the SNP regularization matrix, we employ a similar approach but, instead of spatial proximity, use the linkage disequilibrium between SNPs. We normalize each row of the regularization matrices such that they sum to one.

*Regularization and initialization parameter setting:* Because we have a clear train-test split — and our ultimate goal is to relate brain structure and SNPs to clinical scores of anxiety and depression — we are able to select parameters based on (1) data-driven measurements, (2) prior knowledge and (3) the minimum total SiMLR energy over several different initializations. First, data-driven analysis from a helper function given in the examples above (and as described in[7]) suggests we choose a rank of 99 bases. This is likely to be overparameterized (given the regularization and the noise associated with SNPs) and, as such, we only perform inferential testing in a subset of these bases (strategy described below). Second, prior knowledge informs the selection of regularization matrix parameters, as described in previous sections. We tune the regularization matrices such that the solutions, $V_i$, represent plausibly smooth neuroanatomical networks when represented in the image/brain space. Using (3) is akin to a multi-start optimization method which reduces sensitivity to local minima. We search over 20 initial starting solutions and select the one with the best variance explained as the source of basis functions for application to the test data. After selecting the best model from the multi-start, we select the number of components to test. To assist this, we use `ANTsR` function `predictSiMLR` which summarizes the predictive capacity of each component for each modality. Several summary measures are included, in particular overall variance explained (averaged over all entries in each matrix) and the mean $t$-statistic for each component. As shown in Figure 3, we then plot the mean $t$-statistic over each component set i.e. the mean of ( thickness component-$k$-$t$—statistic + FA component-$k$-$t$—statistic + SNP component-$k$-$t$—statistic ). Inspecting this curve shows relatively little improved descriptive capability beyond 20 components/embeddings. We therefore test for associations between

embeddings and anxiety/depression outcomes in the first 20 components.

## 2.2 Results

### 2.2.1 Relevance of low-dimensional embeddings to depression and anxiety

SiMLR is applied, above, as an unsupervised dimensionality reduction method operating on thickness, FA and SNPs. The resulting components can then be tested, inferentially, for associations with other measurements which we do, here, in an independent sub-cohort of PING. The key to such an approach is that none of the target outcome data is visible to the dimensionality reduction algorithm. An analogous traditional method is principal component regression.

We adopt a step-wise procedure to determine whether the SiMLR component regression demonstrates association with anxiety or depression scores. We assess the following candidate models in testing data:

- m-b: the base model is CES-DC or AED $\approx age + gender + pedu + inc + gaf + scanner$ where *pedu* indicates parental educational level (in years) and *inc* denotes parental income. Four scanner types are included as factors to mitigate the effect of scanner variability. Six genetic ancestry factors are also included via the *gaf* variables. These control for potential ethnic or racial differences in the population sampling.
- m-f: adds $X_{\text{thickness}}V^k_{\text{thickness}}$, $X_{\text{FA}}V^k_{\text{FA}}$ and $X_{\text{SNPs}}V^k_{\text{SNPs}}$ as predictors to m-b.

We assess such models for each $k$ (i.e. over the 20 sets of triplet components) and compute empirical $p$-values by permutation. I.e. we test the ANOVA(m-b,m-f) $F$-score in the original data and compare the result to the same model but in permuted data. This gives insight as to whether the additional set of basis vectors augments predicton while accounting for loss of degrees of freedom. Figure 3 panel (d) shows a scatter-plot of the prediction and the variance explained for the m-f model of AED. We perform 5,000 permutations for each $k$. The table of permutation-based $p$-values for each score and each component is in supplementary Table 2. For the best component (11), permutation-based assessment leads to a $p$-value of 0.0 (effectively $<$ 2e-4) for anxiety and 0.0026 for the depression scores. "Best" is defined, here, as relating significantly to anxiety and depression. The empirical $p$-values derive from the frequency at which the permuted embedding model performance exceeds the omnibus model from original data. No instance of the permuted embeddings exceeded the original data for anxiety scores.

Results are shown in Table 2 and indicate that a subset of embeddings contributes predictive value for both AED and CES-DC, in particular for components 6, 11, 14. Investigating the raw regression models suggests that FA does not add substantial value to the score prediction. SNPs and thickness are consistently useful in both cases. Note that this is a post-hoc observation in that we have not explicitly tested for the significance of thickness versus SNPs or FA. We only test the triplets as a group. Two nuisance predictors reach marginal significance with age and GAF3 at $p$-value 0.014.

Supplementary Table 2: Three SiMLR components survive correction for multiple comparisons out of 20 (components columns). p-Val-Dep indicates raw permutation-based $p$-values for the depression score. q-Val-Dep indicates Bonferroni corrected $p$-values. p-Val-Anx indicates raw permutation-based $p$-values for the anxiety score with $q$ indicating Bonferroni correction. Only a single component – less significant than those derived from SiMLR – survives the same procedures when SGCCA is used for dimensionality reduction.

| method | component | p.Val.Dep | q.Val.Dep | p.Val.Anx | q.Val.Anx |
|---|---|---|---|---|---|
| SiMLR | 6 | 0.003801 | 0.07602 | 2e-04 | 0.004 |
| SiMLR | 11 | 0.002601 | 0.05201 | 2e-04 | 0.004 |
| SiMLR | 14 | 0.006401 | 0.128 | 0.0018 | 0.03601 |
| SGCCA | 4 | 0.0194 | 0.388 | 0.0024 | 0.04801 |

#### 2.2.2 Comparison to SGCCA

As in the main text, we perform the same analysis with SGCCA where we use analogous parameters for that method. Computation time for SGCCA to arrive at convergence was $\approx$ 26 hours using a 2.4 GHz 8-Core Intel Core i9 processor. SiMLR, on the other hand, converged in under an hour.

We also performed statistical testing in the same manner as above but with SGCCA embeddings. Only one component was related to anxiety after multiple comparisons correction. However, the model fit to anxiety scores was relatively consistent with SiMLR although somewhat weaker from the perspective of permutation-tested significance.

#### 2.2.3 Visualization/interpretation of cortical regions

Sparse methods have the value of balancing the exploratory spirit of traditional machine learning tools (e.g. SVD) while retaining some of the interpretability and localization of hypothesis-driven (or univariate) designs. In the current example, we gain interpretability by being able to visualize the embedding vectors in the cortical and white matter spaces, respectively, as in Figure 4. In the case of the brain, as in SNPs, identifying the anatomical location of the weights of the embedding vectors can yield further insight. Table 3 shows a breakdown of the relative anatomical contributions and locations of the weighted anatomy in the most predictive thickness embeddings. Cingulate cortex, precuneus and insula emerge as the most highly weighted regions. These regions have all been implicated in several prior studies of depression and cortical anatomy[8]. Of these, insula and cingulate cortex are reported to have the greatest relationship to clinical symptoms (Table 1 in[8]). Furthermore, note that our choice of the regularization matrices guarantees that the selected feature signal is smooth across each modality's feature space. This process gives a smoothly varying embedding vector (as can be seen in the brain spaces in Figure 4) and prevents over-fitting

and isolated non-plausible high-weight entries. The same method can be used for white matter regions although white matter is not typically as closely associated with specific cognitive domains. As such, we do not pursue this further.

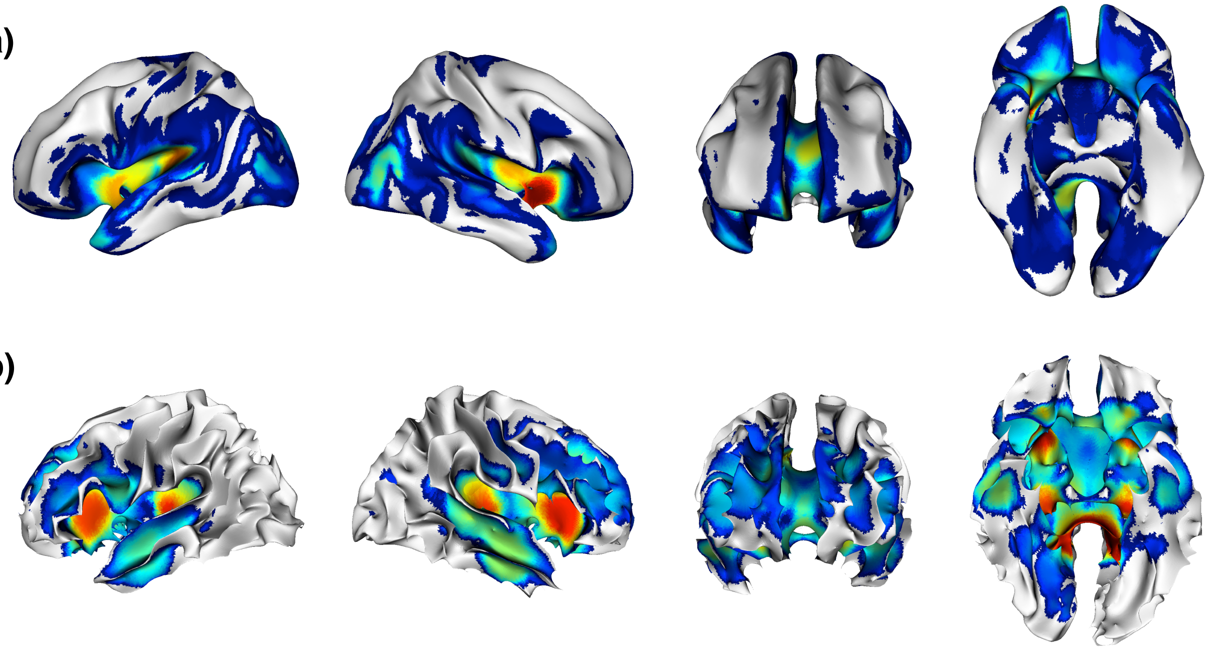


Supplementary Figure 4: Visualization of high-dimensional embedding vectors. Panel (a) shows the most predictive thickness high-dimensional embedding vector. Panel (b) shows the same for the FA. High weights should not be over-interpreted as they may represent algorithmic constraints as well as relevance to the representation.

Supplementary Table 3: The anatomical coordinates and feature weights of the primary cortical embedding vector. The column entitled *weightedVolume* indicates the volume of the region multiplied by the feature weight vector; as such, this is a surrogate for its contribution to the embedding (low-dimensional projection) associated with this feature vector. Over half of the signal is attributable to the left and right insula, cingulate cortices and the precuneus. MNI coordinates are also reported. Anatomical labels are derived from the AAL label set in `ANTsR` (see `data(aal)` )[9]. `cwts` refers to the cumulative contribution of the regions including and preceding the given row. `weightedVolume` is in $mm^3$. A similar table could be constructed for embedding vectors related to the SNP data.

| anat | weightedVolume | cwts | coord.1 | coord.2 | coord.3 |
|---|---|---|---|---|---|
| Cingulum_Ant_R | 5175 | 0.1294 | -7.022 | -37.05 | 13.68 |

| anat | weightedVolume | cwts | coord.1 | coord.2 | coord.3 |
|---|---|---|---|---|---|
| Cingulum_Ant_L | 4601 | 0.2445 | 5.193 | -36.57 | 11.53 |
| Cingulum_Mid_L | 3725 | 0.3377 | 4.841 | 28.03 | 38.3 |
| Precuneus_L | 3311 | 0.4205 | 5.197 | 53.98 | 38.56 |
| Precuneus_R | 2189 | 0.4753 | -6.499 | 51.69 | 43.8 |
| Insula_R | 1908 | 0.523 | -35.82 | -3.142 | 8.851 |
| Cingulum_Mid_R | 1876 | 0.5699 | -5.916 | 6.93 | 37.19 |
| Frontal_Med_Orb_R | 1686 | 0.6121 | -5.415 | -44.39 | -8.303 |
| Insula_L | 1634 | 0.6529 | 35.79 | -0.07309 | 7.716 |
| Frontal_Inf_Tri_L | 1314 | 0.6858 | 42.86 | -29.13 | 1.505 |
| Rectus_L | 934.9 | 0.7092 | 5.387 | -30.29 | -21.72 |
| Frontal_Sup_Medial_L | 767.1 | 0.7284 | 8.051 | -46.64 | 15.94 |
| Fusiform_L | 756.6 | 0.7473 | 33.51 | 25.85 | -27.85 |

### 2.2.4 Interpretation of genetic regions

The source meta-analysis[1] supplies genetic regions for this study that are a priori related to major depressive disorder (MDD). As such, whatever SNPs are identified by SiMLR already have known associations with MDD. Furthermore, Wray et al. provide detailed background for each of the 44 genetic regions that they identify and note that their effects are likely both quantitative and polygenic; i.e. not isolated to a single SNP.

One avenue to interpreting SiMLR feature extraction is to identify, for a given SNP-related SiMLR component, the weight distribution across the source genetic region. As we showed for the brain, this would suggest the regions that are most represented by the sparse selection mechanism. Indeed, in both components 6 and 11, the same region is robustly represented: chromosome 6: from 27,737,591 bp to 32,847,591 bp. They provide – in supplementary Table 6 – the previously identified functions of this and other regions. For this region, they report:

> "There are multiple significant SNPs across two large segments of the extended Major Histocompatibility Complex (MHC) region, as is also observed for schizophrenia (PMID 25056061), but this is a gene-rich region with extensive LD making interpretation of common SNP data difficult."

Nevertheless, our current analysis suggests that the region may indeed be worth further investigation for its role in anxiety and depression.

The second most prominent region is chr 9: 11,066,964-11,846,964. The authors note:

> The associated region is within a 2 Mb intergenic region flanked by PTPRD (Protein Tyrosine Phosphatase, Receptor type D) and TYRP1 (Tyrosinase-Related Protein 1). Bioinformatic analyses (PMID 22649255) indicate little transcriptional activity around the lead SNP (DNAseI hypersensitivity, histone or transcription factor binding or chromatin interactions). PTPRD is highly expressed in brain and is implicated in neural development and in cancer and diabetes (PMID 15674434). In mice, PTPRD plays important roles in axon guidance,

termination and myelination, and synapse and mitral cell dendrite formation (PMID 27026654; 26341907; 16738228). In humans, PTPRD SNPs are associated with restless leg syndrome and with addiction-related behaviors; follow-up work in mice suggests an association between reduced PTPRD expression and behaviors including locomotion, sleep and cocaine-conditioned place preference (PMID 26181631). TYRP1 is specifically expressed in melanocytes and involved in the production of melanin, primarily by maintaining the stability and levels of tyrosine in the melanosome (PMID 9822646; 11775055).

We share this information, here, in order to clarify that interpretation remains complex even in the context of meta-analyses. Larger datasets will be needed in order to provide more concrete and predictive modeling relating genes, environment, behavior and any intermediate mediation that may occur in the brain.

# 3 Genetic risk in Alzheimer's disease

The Alzheimer's disease neuroimaging initiative (ADNI) distributes multi-omic data in healthy elderly, mild cognitive impairment and Alzheimer's disease subjects ages 55 to 90. As of summer 2020, we obtained aggregate data that span ADNI-1, ADNI-2, ADNI-GO and ADNI-3 and that summarizes a variety of measurements in 2,269 subjects. Data is available at http://adni.loni.usc.edu.

A polygenic hazard score (PHS) and related measurements were added to ADNI as the result of recent work by the Desikan lab[10–12]. These measurements are also available at the above link. The PHS is derived from 17,008 AD cases and 37,154 controls from the International Genomics of Alzheimer's Project and is based on a Cox proportional hazards model that predicts risk for AD conversion. We merged both the PHS and the cumulative incidence rate (CIR) into the omnibus data file to enable a multi-omics study.

The PHS models the cumulative genetic risk for AD which includes but also goes beyond the apolipoprotein E type 4 (APOE4) allele. Evaluation of the PHS with respect to in vivo markers of AD-related pathology affirmed that "amyloid and total tau positivity systematically varies as a function of PHS"[11]. Furthermore,[12] showed additional relationships with both longitudinal atrophy and cognitive decline. The success of the PHS in predicting age of onset for sporadic AD demonstrates that it may indeed capture distributed genetic risk. However, PHS may also capture disease processes beyond pure AD as it also correlates with cerebrovascular pathology and presence of Lewy body pathology [3].

## 3.1 Study design

In this evaluation, we will use dimensionality reduction methods to build low-dimensional models predicting PHS from disparate modalities. We use dimensionality reduction as a supervised learning method for integrating several objective measurements to predict a lower-dimensional variable, the PHS for each individual in a test set.

### 3.1.1 Data description

These multi-view matrices include:

- volumetric (structural) MRI measures of the hippocampus, ventricles, whole brain, entorhinal cortex, fusiform cortex and middle temporal cortex ($p$=6);
- AD-relevant cognitive metrics totaling $p = 17$ predictors (shown in Table 1);

Supplementary Table 4: Mean and standard deviation of the cognitive variables used in this study (SMC diagnosis excluded).

| | CN | MCI | AD |
|---|---|---|---|
| **EcogSPMem.bl** | 1.25 +/- 0.37 | 2.20 +/- 0.79 | 3.29 +/- 0.62 |
| **EcogSPLang.bl** | 1.11 +/- 0.22 | 1.66 +/- 0.67 | 2.47 +/- 0.77 |
| **EcogSPVisspat.bl** | 1.05 +/- 0.13 | 1.42 +/- 0.58 | 2.39 +/- 0.85 |
| **EcogSPPlan.bl** | 1.10 +/- 0.29 | 1.56 +/- 0.69 | 2.62 +/- 0.82 |
| **EcogSPOrgan.bl** | 1.14 +/- 0.39 | 1.64 +/- 0.74 | 2.86 +/- 0.85 |
| **EcogSPDivatt.bl** | 1.25 +/- 0.46 | 1.90 +/- 0.83 | 3.02 +/- 0.88 |
| **EcogSPTotal.bl** | 1.15 +/- 0.24 | 1.74 +/- 0.61 | 2.76 +/- 0.63 |
| **MMSE.bl** | 29.0 +/- 1.15 | 28.0 +/- 1.71 | 23.1 +/- 2.05 |
| **mPACCdigit** | -0.1 +/- 2.75 | -5.4 +/- 4.16 | -16. +/- 3.39 |
| **ADAS11.bl** | 5.86 +/- 3.10 | 9.35 +/- 4.41 | 20.6 +/- 6.86 |
| **ADAS13.bl** | 9.20 +/- 4.52 | 15.0 +/- 6.77 | 30.9 +/- 8.07 |
| **ADASQ4.bl** | 2.93 +/- 1.85 | 5.06 +/- 2.62 | 8.68 +/- 1.44 |
| **LDELTOTAL.bl** | 13.5 +/- 3.04 | 7.18 +/- 3.16 | 1.49 +/- 1.76 |
| **CDRSB.bl** | 0.03 +/- 0.13 | 1.46 +/- 0.89 | 4.48 +/- 1.62 |
| **mPACCtrailsB** | -0.0 +/- 2.58 | -4.5 +/- 3.71 | -14. +/- 3.30 |
| **RAVLT.immediate.bl** | 45.5 +/- 10.2 | 36.8 +/- 10.9 | 22.0 +/- 6.80 |
| **RAVLT.learning.bl** | 5.83 +/- 2.39 | 4.65 +/- 2.58 | 1.75 +/- 1.71 |

- molecular measurements of glucose metabolism (via fluorodeoxyglucose (FDG)-positron emission tomography (PET)), amyloid levels (via cerebrospinal fluid assays and AV45 PET (florbetapir)), tau and phosphorylated tau levels from cerebrospinal fluid ($p$=5);
- genetic risk for AD (the supervising matrix) composed of the APOE4 allele (a trinary value in 0,1,2), the PHS and the CIR.

Subjects in this study were required to have all of the above modalities. This resulted in 723 (n=335 female) unique individuals with baseline diagnosis of either control (n=137), subjective memory complaint (n=80), MCI (n=391) or AD (n=115) with age 72.55 $\pm$ 7.2. The mean MMSE at baseline in each diagnostic group is shown in table 1. Specific RIDs for the included subjects appear toward the end of this report.

This complete dataset, relative to our other evaluation studies, is more classical in the sense

that $n >> p$. As such, sparseness is perhaps less critical to preventing overfitting and for interpretation. We therefore compare SiMLR *without sparseness* to RGCCA as well as SGCCA and SiMLR variants *with sparseness*.

### 3.1.2 Evaluation of PHS prediction

Dimensionality reduction across the joint space of brain structure, cognition and molecular signatures of disease (amyloid and tau - the known primary pathological vectors as well as a measure of glucose metabolism, FDG PET) should lead to an approximation of the latent AD space, especially with the direct supervision of PHS, CIR and APOE4 genotype. The polygenic risk for AD will serve as a proxy for the true latent space, which cannot be known. As such, we do not expect to predict the PHS exactly but to find a latent space that is at least related to the PHS:

> we assess the success of this learning process via cross-validation i.e. 150 training-testing splits of the data (80% of data in training set) with learning and evaluation results being tabulated at each split. This permits a paired $t$-test on the $R^2$ of the predicted PHS to the real PHS to compare the methods.

This study design effectively inverts the PHS evaluation approach used in [2,3]. We achieve this by jointly decomposing the matrices describing these 4 types of input data ( genetic risk, structure, molecular and cognition ) and then, in a test set, demonstrate that polygenic risk score can be predicted from the latent space of the other 3 modalities. RGCCA, SGCCA and SiMLR perform very closely in this study with SiMLR showing an edge in performance across all settings. Parameters for the methods were matched as closely as is possible for each comparison. Results are in Figure 1 where we note that each run is computed with a different starting seed for the series of cross-validation splits. Additional details follow.

### 3.1.3 Dimensionality reduction parameters

For both SGCCA and SiMLR, we derive two components from the dimensionality reduction, i.e. a rank-2 solution for each modality. We choose a very low-dimensional space for interpretability and because the input matrices are themselves fairly small with the smallest matrix containing only 3 columns (genetic risk). We use default parameters for each method with a sparseness penalty, for SGCCA and SiMLR comparisons, that seeks to zero out roughly half of the feature variables in each matrix. For SiMLR and RGCCA comparisons, we do not use sparseness penalties.

### 3.1.4 Joint prediction of PHS from structure, cognition and molecular predictors

The variable selection listed in the previous section results in low-dimensional predictors that we use in linear regression to predict PHS as an outcome variable. Our baseline model is of the form:

$$\text{PHS} \approx \text{Age} + \text{Gender} + \text{EducationalLevel}$$

with each dimensionality reduction evaluated with an extended model adding a rank-2 matrix of predictors for each modality:

$$\text{PHS} \approx \cdots + \text{structure} + \text{cognition} + \text{molecular}$$

where each predictor above is defined by:

$$\text{predictor} = X_{\text{predictor}} * V_{\text{predictor}},$$

i.e. the low-dimensional representation of each data matrix. A better latent representation should result in a better prediction of PHS in the test data.

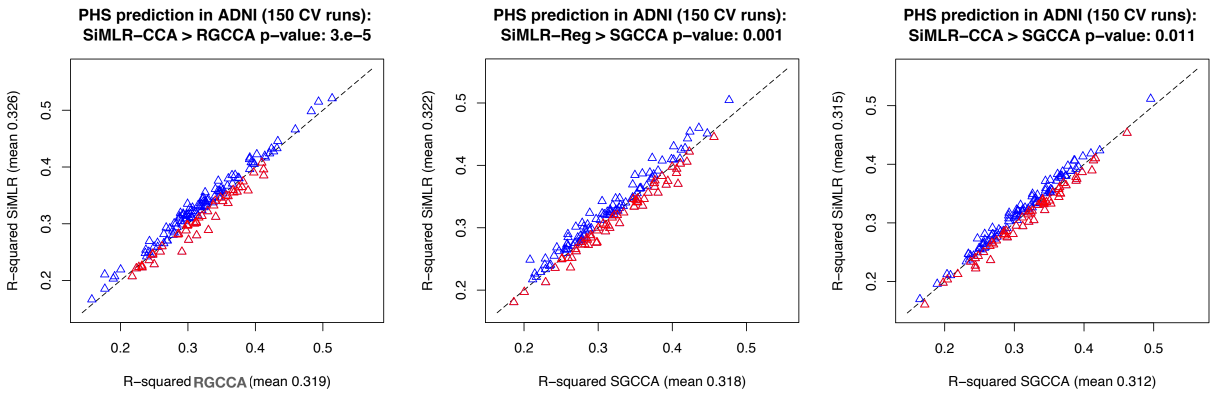


Supplementary Figure 5: Cross-validation results: SiMLR-CCA (no sparseness) vs RGCCA (left), SiMLR-Regression (default sparseness) vs SGCCA (same sparseness as SiMLR) (center) and SiMLR-CCA (default sparseness) vs SGCCA (same sparseness as SiMLR) (right). For all panels, the blue/red triangles represent points where SiMLR yields a better/worse result than RGCCA or SGCCA. Relatedly, points above the dotted line occur when SiMLR exhibits better performance.

#### 3.1.5 Data usage

Data used in the preparation of this report were obtained from the Alzheimer's Disease Neuroimaging Initiative (ADNI) database (adni.loni.usc.edu). The ADNI was launched in 2003 as a public-private partnership, led by Principal Investigator Michael W. Weiner, MD. The primary goal of ADNI has been to test whether serial magnetic resonance imaging (MRI), positron emission tomography (PET), other biological markers, and clinical and neuropsychological assessment can be combined to measure the progression of mild cognitive impairment (MCI) and early Alzheimer's disease (AD). For up-to-date information, see www.adni-info.org.

#### 3.1.6 ADNI subject ids

The following RIDs were used at the baseline visit in this study.

```
## Participant roster ID
##   [1] 2002 2010 2018 2022 2026 2027 2031 2036 2042 2045 2047 2052 2055 2058 2060
##  [16] 2061 2063 2068 2072 2073 2074 2079 2083 2087 2093 2099 2100 2106 2116 2119
##  [31] 2121 2124 2125 2130 2133 2142 2146 2148 2150 2151 2153 2155 2164 2167 2168
##  [46] 2171 2180 2182 2183 2185 2187 2190 2193 2194 2195 2196 2199 2201 2208 2210
##  [61] 2213 2216 2219 2220 2225 2233 2234 2238 2240 2245 2247 2249 2263 2264 2274
##  [76] 2301 2304 2307 2308 2315 2316 2332 2333 2336 2347 2357 2360 2363 2367 2373
##  [91] 2374 2378 2380 2381 2390 2391 2394 2396 2398 2403 2407 4001 4003 4004 4005
## [106] 4007 4010 4012 4014 4015 4018 4020 4022 4024 4026 4028 4029 4034 4035 4036
## [121] 4037 4039 4041 4042 4043 4050 4053 4057 4058 4059 4060 4061 4063 4066 4067
## [136] 4072 4073 4075 4076 4077 4079 4080 4081 4082 4084 4086 4089 4090 4092 4093
## [151] 4094 4096 4100 4102 4103 4104 4105 4114 4115 4119 4120 4121 4122 4125 4127
## [166] 4128 4131 4133 4134 4138 4139 4143 4146 4148 4149 4150 4151 4152 4153 4157
## [181] 4158 4159 4160 4162 4164 4167 4168 4170 4171 4172 4173 4174 4175 4176 4177
## [196] 4179 4184 4185 4187 4188 4189 4192 4194 4195 4196 4197 4198 4199 4200 4201
## [211] 4202 4203 4205 4206 4208 4209 4210 4211 4213 4214 4215 4217 4218 4219 4220
## [226] 4223 4224 4225 4226 4229 4232 4235 4237 4240 4241 4243 4244 4250 4251 4252
## [241] 4254 4256 4258 4262 4263 4266 4268 4269 4270 4271 4272 4274 4275 4276 4278
## [256] 4280 4281 4282 4285 4288 4290 4291 4292 4293 4294 4299 4300 4301 4302 4303
## [271] 4308 4310 4311 4312 4320 4324 4331 4332 4335 4337 4338 4339 4340 4343 4346
## [286] 4348 4349 4350 4351 4352 4353 4354 4356 4357 4359 4360 4363 4365 4366 4367
## [301] 4369 4371 4376 4377 4379 4381 4382 4384 4386 4387 4388 4390 4391 4392 4393
## [316] 4394 4396 4399 4401 4402 4404 4405 4406 4408 4410 4414 4415 4417 4420 4421
## [331] 4422 4424 4426 4428 4429 4430 4431 4433 4434 4438 4443 4444 4445 4447 4448
## [346] 4449 4453 4455 4456 4458 4462 4463 4464 4465 4466 4467 4468 4469 4473 4474
## [361] 4475 4477 4480 4482 4485 4488 4489 4491 4494 4496 4498 4499 4500 4501 4502
## [376] 4503 4505 4506 4507 4508 4510 4512 4513 4514 4515 4516 4517 4520 4521 4522
## [391] 4524 4526 4530 4536 4538 4539 4540 4542 4543 4545 4546 4547 4548 4549 4552
## [406] 4553 4557 4560 4562 4565 4566 4568 4571 4578 4580 4582 4583 4584 4585 4586
## [421] 4587 4589 4590 4591 4594 4595 4596 4597 4598 4599 4604 4605 4611 4612 4613
## [436] 4615 4616 4621 4623 4624 4625 4626 4629 4630 4631 4635 4637 4638 4641 4643
## [451] 4645 4646 4653 4654 4657 4659 4661 4668 4672 4674 4675 4676 4678 4679 4680
## [466] 4686 4688 4689 4692 4694 4706 4707 4708 4711 4712 4713 4714 4715 4718 4720
## [481] 4721 4723 4728 4729 4730 4732 4736 4737 4739 4741 4743 4744 4745 4746 4750
## [496] 4755 4756 4757 4764 4765 4767 4770 4774 4777 4780 4782 4783 4784 4785 4793
## [511] 4796 4801 4802 4803 4804 4805 4806 4807 4809 4813 4814 4815 4816 4817 4823
## [526] 4825 4835 4842 4845 4849 4852 4853 4856 4857 4858 4859 4862 4863 4867 4868
## [541] 4869 4871 4874 4876 4879 4885 4887 4889 4893 4894 4896 4897 4898 4899 4903
## [556] 4904 4905 4906 4907 4909 4910 4911 4917 4918 4919 4920 4922 4924 4925 4926
## [571] 4928 4929 4936 4940 4941 4943 4944 4945 4947 4949 4954 4955 4958 4959 4960
## [586] 4962 4964 4966 4971 4974 4976 4980 4982 4984 4986 4987 4989 4990 4992 4994
## [601] 4997 5000 5004 5006 5012 5013 5014 5017 5018 5019 5026 5027 5028 5029 5031
## [616] 5038 5054 5059 5062 5063 5067 5070 5078 5079 5082 5083 5087 5090 5091 5093
## [631] 5095 5096 5097 5099 5100 5102 5106 5109 5110 5112 5113 5118 5120 5121 5123
## [646] 5124 5125 5127 5135 5141 5142 5147 5150 5153 5154 5157 5159 5160 5162 5165
```

```
## [661] 5167 5169 5170 5171 5175 5176 5177 5178 5185 5193 5194 5195 5196 5197 5198
## [676] 5202 5203 5204 5205 5208 5209 5210 5213 5214 5218 5219 5222 5224 5227 5228
## [691] 5231 5234 5236 5237 5241 5242 5244 5248 5251 5252 5253 5256 5258 5259 5261
## [706] 5263 5265 5266 5267 5269 5271 5272 5275 5277 5278 5279 5283 5287 5288 5289
## [721] 5290 5292 5295
```

#### 3.1.7 Data files

- ADNIMERGE in `R`
- `DESIKANLAB.csv` from LONI

#### 3.1.8 Acknowledgments

Data collection and sharing for this project was funded by the Alzheimer's Disease Neuroimaging Initiative (ADNI) (National Institutes of Health Grant U01 AG024904) and DOD ADNI (Department of Defense award number W81XWH-12-2-0012). ADNI is funded by the National Institute on Aging, the National Institute of Biomedical Imaging and Bioengineering, and through generous contributions from the following: AbbVie, Alzheimer's Association; Alzheimer's Drug Discovery Foundation; Araclon Biotech; BioClinica, Inc.; Biogen; Bristol-Myers Squibb Company; CereSpir, Inc.; Eisai Inc.; Elan Pharmaceuticals, Inc.; Eli Lilly and Company; EuroImmun; F. Hoffmann-La Roche Ltd and its affiliated company Genentech, Inc.; Fujirebio; GE Healthcare; IXICO Ltd.; Janssen Alzheimer Immunotherapy Research & Development, LLC.; Johnson & Johnson Pharmaceutical Research & Development LLC.; Lumosity; Lundbeck; Merck & Co., Inc.; Meso Scale Diagnostics, LLC.; NeuroRx Research; Neurotrack Technologies; Novartis Pharmaceuticals Corporation; Pfizer Inc.; Piramal Imaging; Servier; Takeda Pharmaceutical Company; and Transition Therapeutics. The Canadian Institutes of Health Research is providing funds to support ADNI clinical sites in Canada. Private sector contributions are facilitated by the Foundation for the National Institutes of Health (www.fnih.org). The grantee organization is the Northern California Institute for Research and Education, and the study is coordinated by the Alzheimer's Disease Cooperative Study at the University of California, San Diego. ADNI data are disseminated by the Laboratory for Neuro Imaging at the University of Southern California.

Data used in preparation of this article were obtained from the Alzheimer's Disease Neuroimaging Initiative (ADNI) database (adni.loni.usc.edu). As such, the investigators within the ADNI contributed to the design and implementation of ADNI and/or provided data but did not participate in the analysis or writing of this report. A complete listing of ADNI investigators can be found at: http://adni.loni.usc.edu/wp-content/uploads/how_to_apply/ADNI_Acknowledgment_List.pdf

# References

1. Wray, N. R. *et al.* Genome-wide association analyses identify 44 risk variants and refine the genetic architecture of major depression. *Nature Genetics* (2018) doi:10.1038/s41588-018-0090-3.

2. Jernigan, T. L. *et al.* The Pediatric Imaging, Neurocognition, and Genetics (PING) Data Repository. *NeuroImage* (2016) doi:10.1016/j.neuroimage.2015.04.057.

3. Tustison, N. *et al.* Large-scale evaluation of ANTs and FreeSurfer cortical thickness measurements. *NeuroImage* **99**, (2014).

4. Avants, B. *et al.* The pediatric template of brain perfusion. *Scientific data* **2**, (2015).

5. Purcell, S. *et al.* PLINK: A Tool Set for Whole-Genome Association and Population-Based Linkage Analyses. *The American Journal of Human Genetics* (2007) doi:10.1086/519795.

6. Avants, B. *Relating high-dimensional structural networks to resting functional connectivity with sparse canonical correlation analysis for neuroimaging.* vol. 136 (2018).

7. O'Connell, M. J. & Lock, E. F. R.JIVE for exploration of multi-source molecular data. *Bioinformatics* (2016) doi:10.1093/bioinformatics/btw324.

8. Schmaal, L. *et al.* Cortical abnormalities in adults and adolescents with major depression based on brain scans from 20 cohorts worldwide in the ENIGMA Major Depressive Disorder Working Group. *Molecular Psychiatry* (2017) doi:10.1038/mp.2016.60.

9. Tzourio-Mazoyer, N. *et al.* Automated anatomical labeling of activations in SPM using a macroscopic anatomical parcellation of the MNI MRI single-subject brain. *Neuroimage* **15**, 273–289 (2002).

10. Desikan, R. S. *et al.* Genetic assessment of age-associated alzheimer disease risk: Development and validation of a polygenic hazard score. *PLoS medicine* **14**, e1002258 (2017).

11. Tan, C. H. *et al.* Polygenic hazard score: An enrichment marker for alzheimer's associated amyloid and tau deposition. *Acta neuropathologica* **135**, 85–93 (2018).

12. Tan, C. H. *et al.* Polygenic hazard score, amyloid deposition and alzheimer's neurodegeneration. *Brain* **142**, 460–470 (2019).
